# Supplementary material for: Improving Attention Mechanism with Query-Value Interaction
Source: arXiv:2010.03766 source file (2020-10-08)
Supplement: Supplementary file 1 [file supplement.tex]

\section*{Appendix}

\subsection*{Experiment Environment}
The configurations of environments for experiments are described as follows.
The machine we used for experiments contains an Intel Xeon E5-2620 v4 CPU, and a GeForce GTX1080Ti GPU.
The total memory is 64GB, and each experiment is run on a single GPU and CPU core with a single process/thread.
The operating system is Ubuntu 16.04 and the programming language is Python (version 3.7).
We use the Keras\footnote{https://github.com/keras-team/} framework with tensorflow 1.12\footnote{https://github.com/tensorflow/tensorflow/releases/tag/v1.12.0} backend to implement deep learning models.

\subsection*{Preprocessing}
On the \textit{AG} dataset, we concatenate the title and description of each news article.
On the \textit{Amazon} dataset, we only use the review body.
We use the NLTK tool\footnote{http://www.nltk.org/} for text tokenization.
On the \textit{Bakeoff-3} and \textit{Bakeoff-4} datasets, we use the BIO tagging scheme to construct labeled samples.

\subsection*{Hyperparameter Settings}
The hyperparameters involved in different methods are listed in Table~\ref{hyper}.

\begin{table}[h]
\centering
\resizebox{0.9\linewidth}{!}{
\begin{tabular}{|l|c|}
\hline
\multicolumn{1}{|c|}{\textbf{Hyperparameters}}& \textbf{Value} \\ \hline
word embedding dimension                     & 300            \\
\# heads in self-attention networks                 & 16             \\
output dim of self-attention head               & 16            \\
\# self-attention layers               & 2            \\
\# CNN filters            & 256            \\
dim of LSTM hidden states              & 256            \\
 dim of additive attention query             & 256          \\
dropout ratio                       & 0.2            \\
optimizer                                    & Adam           \\
learning rate                                & 1e-3           \\
batch size                                   & 64    \\          \hline
\end{tabular}
}
\caption{Detailed settings of hyperparameters.}\label{hyper}
\end{table}

\subsection*{Complementary Experimental Results}
The performance of several attention-based methods using different $g(\mathbf{Q},\mathbf{V})$ on the \textit{Amazon} dataset is
shown in Fig.~\ref{fig.fuse2}.
\begin{figure}[!t]
	\centering
%\subfigure[\textit{AG} dataset.]{
		\includegraphics[width=0.48\textwidth]{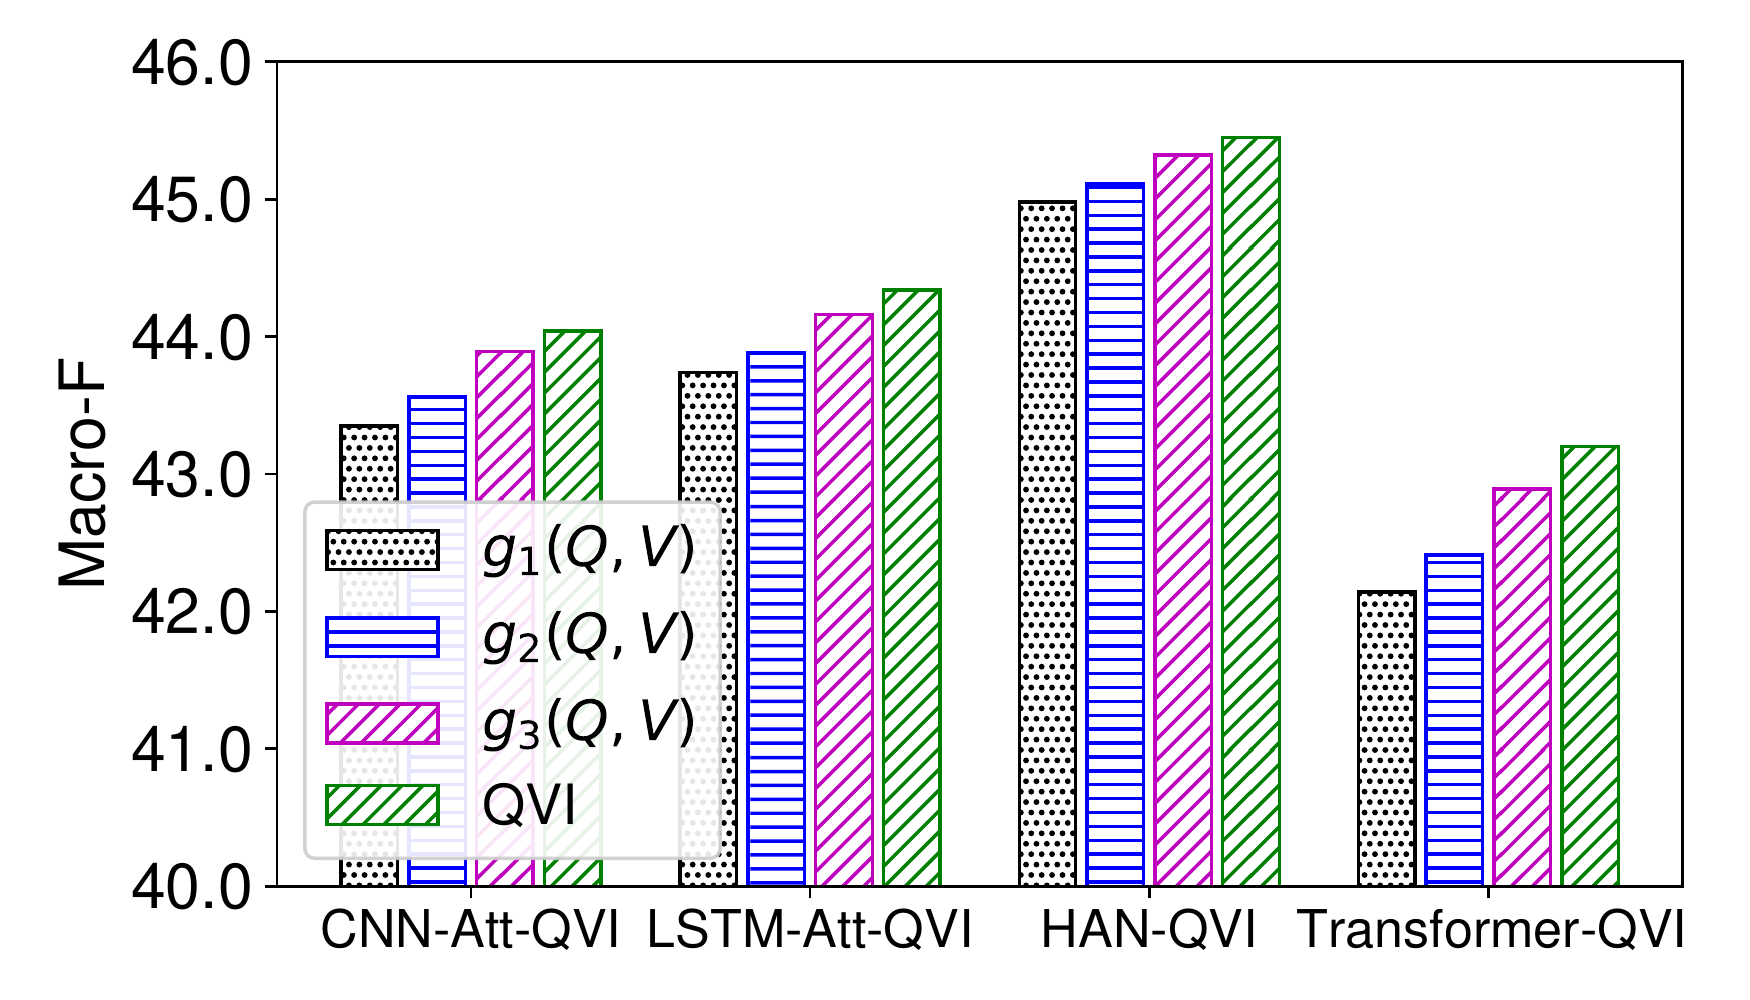}
	%	\subfigure[\textit{Amazon} dataset.]{
		%\includegraphics[width=0.38\textwidth]{fig/fuse.pdf}}
\caption{Influence of QVI modeling on the \textit{Amazon} dataset.}\label{fig.fuse2}
\end{figure}
